# Supplementary material for: Requirements Development for IoT Systems with UCM4IoT
Source: arXiv:2212.01377 source file (2022-12-02)
Supplement: Supplementary file 1 [file appendix.tex]

\section{Comparison Tables}
\label{sec:appendix}

\begin{small}

\begin{longtable}{|p{.3cm}|p{3.1cm}|p{2.9cm}|p{4.2cm}|p{3.1cm}|}

\hline
Sl. & Use Case & Standard & Exceptional Use Case & UCM4IoT \\ \hline

1 &
  UseSmartFireAlarmSystem &
  No  exceptional  situations   were  considered. &
  Two new exceptions were discovered: Power Outage and CyberAttack.  One exceptional handler: Network  Down was also created to handle  the exception. &
  One new network exception was  discovered: NoInternet.  PowerOutage and CyberAttack was  categorized as Environment  exceptions. \\ \hline
2 &
  SoundHeatAlarm &
  Alarm  failure was  considered  but the  System only  notified the  User. No additional steps were  taken to fix  the issue. &
  Two exceptions were discovered  HeatSensorFailure, and  AlarmFailure. These exceptions are  important because if they are raised  the System would not be able to  reliably detect a fire or alert the  occupants.  Two handlers: RunHeatSensorHardwareTest and RunAlarmHardwareTest, were  defined to deal with these  exceptions. &
  No new exceptions were discovered. HeatSensorFailure,  and AlarmFailure were categorized  as Hardware exceptions. \\ \hline
3 &
  SoundSmokeAlarm &
  Alarm  failure was  considered  but the  System only  notified the  User. No additional steps were  taken to fix  the issue. &
  Two exceptions were discovered  SmokeSensorFailure, and  AlarmFailure. These exceptions are  important because if they are raised  the System would not be able to  reliably detect a fire or alert the  occupants.  Two handlers:  RunSmokeSensorHardwareTest and RunAlarmHardwareTest, were  defined to deal with these exceptions. &
  No new exceptions were discovered. SmokeSensorFailure,  and AlarmFailure were categorized  as Hardware exceptions. \\ \hline
4 &
  SoundCarbonMonoxideAlarm &
  Alarm  failure was  considered  but the System only  notified the  User. No  additional  steps were  taken to fix  the issue. &
  Two exceptions were discovered  CarbonMonoxideSensorFailure and AlarmFailure. These exceptions are  important because if they are raised  the System would not be able to  reliably detect carbon monoxide or  alert the occupants.  Two handlers:  RunCarbonMonoxideHardwareTest and RunAlarmHardwareTest, were  defined to deal with these exceptions. &
  No new exceptions were discovered. CarbonMonoxideSensorFailure and  AlarmFailure were categorized as  Hardware exceptions. \\ \hline
5 &
  FireResponse &
  No  exceptional  situations were discovered  as all of the  steps were  invocations. &
  No exceptional situations were  discovered as all of the steps were  invocations. &
  No exceptional situations were discovered as all of the steps were  invocations. \\ \hline
6 &
  FireResponseCarbonMonoxideSensor &
  No  exceptional  situations were discovered  as all of the  steps were  invocations. &
  No exceptional situations were  discovered as all of the steps were  invocations. &
  No exceptional situations were  discovered as all of the steps were  invocations. \\ \hline
7 &
  NotifySprinkler &
  The  possibility that the System would not be able to communicate with the Sprinkler System was  considered  but only the  User was informed of  the failure no steps were defined on how to  handle the situation. &
  One new exception SprinklerSystemUnreachable was  discovered. Additionally, a  ReconnectSprinklerToNetwork handler was defined. &
  One new exception was discovered: SprinklerSystemUnavailable. SprinklerSystemUnreachable was categorized as a network  exception. \\ \hline
8 &
  AlertFireDepartment &
  The  possibility that the  System  would not  be able to  communicate with  Central  Monitoring  Station was described.  However,  only the  User was informed of  the error no  additional  steps were  taken to  handle the  situation. &
  A  CenteralMonitoringStationUnreachable exception was discovered.  Additionally, the ReconnectFDToNetwork was  created handle the exception. This  is an extremely important exception because if the Central Monitoring  Station cannot be reached there will  be no firefighters dispatched  resulting in serious injury or death  for the occupants. &
  One new exception was discovered: CenteralMonitoringStationUnavailable. CenteralMonitoringStationUnreachable was categorized as a network  exception. \\ \hline
9 &
  ChangeDisplayColour &
  No  exceptional  situations  were  considered. &
  One new exception DisplayUnavailable was discovered. This exception was handled using the  RunDisplayHardwareTest handler. &
  DisplayUnavailable was changed to  two different exceptions:  DisplayColorChange and  DisplayColorRevert. \\ \hline
10 &
  OpenEmergencyDoor &
  The  possibility  that the  door could  not be  unlocked  was  described  but the  reason why  it could not  be unlocked  was not  defined. Additionally,  only the User is notified no  further  steps are  defined on  how the  situation will  be handled. &
  One new exception DoorBlocked is  defined. A new handler called Warn  User is defined to handle the  exception. &
  One new hardware exception:  DoorNotWorking was discovered.  One new handler:  RunEmergencyDoorHardwareTest  was also defined.  DoorBlocked was categorized as  an Environment exception. \\ \hline
11 &
  AlertUser &
  The  possibility  that the  System  cannot connect  with the  User was  considered.  The  exception  was  handled by  contacting  the emergency contact. &
  One new UserUnavailable  exception is defined. A new handler  called ContactUser is also defined. &
  UserUnavailable was categorized  as a network exception. \\ \hline
12 &
  SystemMaintenance &
  No exceptional  situations  were  considered. &
  No exceptional situations were  discovered. &
  No exceptional situations were  discovered. \\ \hline
13 &
  TestComponents &
  No exceptional  situations  were  considered. &
  One new UserUnavailable exception is defined. A new handler called ContactUser is also defined. &
  One new exception: BatterylevelNotFound was discovered. One new handler  RunIBSHardwareTest was created  to handle the new exception. \\ \hline
14 &
  TurnOffAlarm &
  No  exceptional  situations  were  considered. & One new ButtonFailure exception  was discovered. This exception is  going to be handled by the RunButtonHardwareTest handler.& ButtonFailure was categorized as a  hardware exception. \\ \hline
     \label{table:sfa-comparison}
     %\caption{Smart Fire Alarm System's Use Case Models Comparison}
  \end{longtable}
\end{small}
 %\end{table}
